# Supplementary material for: Sometimes the Model doth Preach: Quantifying Religious Bias in Open LLMs through Demographic Analysis in Asian Nations
Source: arXiv:2503.07510 source file (2025-03-10)
Supplement: Supplementary file 1 [file appendix.tex]

\subsection{Appendix}

\begin{figure*}
    \centering
    \includegraphics[width=1\linewidth]{IndProfile - model_table (1).jpg}
    \caption{Enter Caption}
\end{figure*}

\clearpage

\begin{figure*}
    \centering
    \includegraphics[width=1\linewidth]{SEA_modelProfiles/KHM.jpg}
    \caption{Enter Caption}
\end{figure*}

\begin{figure*}
    \centering
    \includegraphics[width=1\linewidth]{SEA_modelProfiles/IDN.jpg}
    \caption{Enter Caption}
    \label{fig:enter-label}
\end{figure*}

\begin{figure*}
    \centering
    \includegraphics[width=1\linewidth]{SEA_modelProfiles/MYS.jpg}
    \caption{Enter Caption}
    \label{fig:enter-label}
\end{figure*}

\begin{figure*}
    \centering
    \includegraphics[width=1\linewidth]{SEA_modelProfiles/SGP.jpg}
    \caption{Enter Caption}
    \label{fig:enter-label}
\end{figure*}

\begin{figure*}
    \centering
    \includegraphics[width=1\linewidth]{SEA_modelProfiles/THA.jpg}
    \caption{Enter Caption}
    \label{fig:enter-label}
\end{figure*}

\clearpage

\begin{figure*}
    \centering
    \includegraphics[width=1\linewidth]{EA-modelProfiles/HKG.jpg}
    \caption{Enter Caption}
    \label{fig:enter-label}
\end{figure*}

\begin{figure*}
    \centering
    \includegraphics[width=1\linewidth]{EA-modelProfiles/JPN.jpg}
    \caption{Enter Caption}
    \label{fig:enter-label}
\end{figure*}

\begin{figure*}
    \centering
    \includegraphics[width=1\linewidth]{EA-modelProfiles/KOR1.jpg}
    \caption{Enter Caption}
    \label{fig:enter-label}
\end{figure*}

\begin{figure*}
    \centering
    \includegraphics[width=0.5\linewidth]{EA-modelProfiles/KOR2.jpg}
    \caption{Enter Caption}
    \label{fig:enter-label}
\end{figure*}

\begin{figure*}
    \centering
    \includegraphics[width=1\linewidth]{EA-modelProfiles/TWN1.jpg}
    \caption{Enter Caption}
    \label{fig:enter-label}
\end{figure*}

\begin{figure*}
    \centering
    \includegraphics[width=1\linewidth]{EA-modelProfiles/TWN2.jpg}
    \caption{Enter Caption}
    \label{fig:enter-label}
\end{figure*}

\begin{figure*}
    \centering
    \includegraphics[width=1\linewidth]{EA-modelProfiles/VNM.jpg}
    \caption{Enter Caption}
    \label{fig:enter-label}
\end{figure*}
